# Supplementary material for: Think-Aloud Verbalizations for Identifying User Experience Problems: Effects of Language Proficiency with Chinese Non-Native English Speakers
Source: arXiv:2202.02970 source file (2022-02-07)
Supplement: Supplementary file 1 [file 10-appendix.tex]

\section{Appendices}
% \begin{table}[h]
%   \caption{Number of actual problems identified in each group}
%   \label{tab:actualproblems}
%   \begin{tabular}{cccc}
%     \toprule
% Problem No.	&	Severity	&	Native	&	Non-native	\\
%     \midrule
% M01	&	1	&	Yes	&	Yes	\\
% M02	&	2	&	Yes	&	Yes	\\
% M03	&	1	&	Yes	&	Yes	\\
% M04	&	1	&	Yes	&	Yes	\\
% M05	&	3	&	Yes	&	Yes	\\
% M06	&	3	&	Yes	&	Yes	\\
% L01	&	1	&	Yes	&	Yes	\\
% L02	&	1	&	Yes	&	Yes	\\
% L03	&	1	&	Yes	&	Yes	\\
% L04	&	1	&	Yes	&	Yes	\\
% L05	&	1	&	-	&	Yes	\\
% L06	&	1	&	-	&	Yes	\\
% B01	&	2	&	Yes	&	Yes	\\
% B02	&	2	&	Yes	&	-	\\
% B03	&	1	&	Yes	&	Yes	\\
% B04	&	1	&	Yes	&	Yes	\\
% B05	&	1	&	Yes	&	Yes	\\
% B06	&	1	&	-	&	Yes	\\
% B07	&	1	&	-	&	Yes	\\
%     \bottomrule
% \end{tabular}
% \end{table} 

%%Language proficiency_Number of verbalization segments
%survey 1 is in appendix?
\begin{table}
  \caption{Participants' feeling about thinking aloud}
  \label{tab:survey1}
  \begin{tabular}{p{0.5cm}|p{6.5cm}}
    \toprule
No.	&	Question	\\
    \midrule
    %overfull 1/3
1	&	How mentally demanding was it for you to think aloud?	\\
2	&	How physically demanding was it for you to think aloud?	\\
3	&	How hurried or rushed was it for you to think aloud?	\\
4	&	How successful were you in thinking aloud while you were working on these tasks?	\\
5	&	How hard did you have to work to accomplish your level of performance in thinking aloud?	\\
6	&	How insecure, discouraged, irritated, stressed, and annoyed were you in thinking aloud?	\\
    \bottomrule
\end{tabular}
\end{table}

%survey 2 is in appendix
\begin{table}
  \caption{Participants' preference on protocols}
  \label{tab:survey2}
  \begin{tabular}{p{0.5cm}|p{6.5cm}}
    \toprule
No.	&	Statements	\\
    \midrule
    %overfull!
1	&	I didn't feel I was interrupted by questions (not tasks) during the session.	\\
2	&	I like the way I was interacted with in the session.	\\
    \bottomrule
\end{tabular}
\end{table}

\begin{table}[hbt!]
  \caption{Not using: Number of verbalization segments in each category for each participant}
  \label{tab:numSegIndi}
  \begin{tabular}{p{0.3cm}|p{1.35cm}|p{1.4cm}|p{0.8cm}|p{1.2cm}|p{1.0cm}}
    \toprule
    ID & Explanation & Observation & Others & Procedure & Reading\\
    \midrule
1	&	10	&	39	&	30	&	38	&	28	\\
2	&	10	&	86	&	81	&	67	&	11	\\
3	&	20	&	142	&	42	&	100	&	44	\\
4	&	1	&	65	&	45	&	72	&	14	\\
5	&	30	&	132	&	90	&	80	&	50	\\
6	&	11	&	52	&	38	&	88	&	9	\\
7	&	14	&	69	&	51	&	74	&	67	\\
8	&	11	&	64	&	47	&	50	&	37	\\
9	&	10	&	164	&	50	&	84	&	47	\\
10	&	17	&	105	&	43	&	110	&	18	\\
11	&	18	&	112	&	48	&	110	&	18	\\
12	&	11	&	49	&	34	&	88	&	21	\\
13	&	14	&	117	&	54	&	90	&	31	\\
14	&	33	&	166	&	45	&	60	&	20	\\
15	&	32	&	69	&	34	&	103	&	31	\\
16	&	18	&	89	&	36	&	97	&	39	\\
17	&	15	&	54	&	40	&	76	&	21	\\
18	&	40	&	83	&	52	&	143	&	46	\\
    \bottomrule
\end{tabular}
\end{table}

\begin{table}[hbt!]%why it's not under section 10?
  \caption{Not using: Number of verbalization segments in each category in CTA}
  \label{tab:numSegCTA}
  \begin{tabular}{p{0.3cm}|p{1.35cm}|p{1.4cm}|p{0.8cm}|p{1.2cm}|p{1.0cm}}
    \toprule
    ID & Explanation & Observation & Others & Procedure & Reading\\
    \midrule
1	&	4	&	18	&	9	&	9	&	15	\\
2	&	5	&	26	&	31	&	48	&	5	\\
3	&	1	&	33	&	15	&	29	&	6	\\
4	&	0	&	31	&	12	&	25	&	3	\\
5	&	8	&	35	&	23	&	13	&	15	\\
6	&	0	&	4	&	7	&	40	&	2	\\
7	&	0	&	10	&	15	&	43	&	15	\\
8	&	3	&	22	&	10	&	11	&	7	\\
9	&	4	&	54	&	19	&	31	&	17	\\
10	&	4	&	36	&	20	&	34	&	9	\\
11	&	5	&	17	&	14	&	52	&	1	\\
12	&	3	&	15	&	11	&	24	&	12	\\
13	&	4	&	54	&	28	&	28	&	14	\\
14	&	6	&	45	&	18	&	15	&	7	\\
15	&	4	&	17	&	10	&	44	&	10	\\
16	&	11	&	20	&	18	&	49	&	12	\\
17	&	3	&	14	&	10	&	6	&	2	\\
18	&	9	&	41	&	14	&	44	&	21	\\
    \bottomrule
\end{tabular}
\end{table}

\begin{table}[hbt!]
  \caption{Not using: Number of verbalization segments in each category in SC}
  \label{tab:numSegSC}
  \begin{tabular}{p{0.3cm}|p{1.35cm}|p{1.4cm}|p{0.8cm}|p{1.2cm}|p{1.0cm}}
    \toprule
    ID & Explanation & Observation & Others & Procedure & Reading\\
    \midrule
    1	&	3	&	9	&	10	&	8	&	7	\\
    2	&	2	&	25	&	25	&	9	&	2	\\
    3	&	1	&	23	&	11	&	42	&	15	\\
    4	&	1	&	11	&	18	&	34	&	5	\\
    5	&	7	&	44	&	40	&	21	&	24	\\
    6	&	4	&	12	&	17	&	16	&	2	\\
    7	&	6	&	12	&	14	&	11	&	20	\\
    8	&	5	&	5	&	15	&	23	&	1	\\
    9	&	5	&	64	&	11	&	17	&	6	\\
    10	&	5	&	22	&	9	&	9	&	1	\\
    11	&	5	&	59	&	18	&	34	&	11	\\
    12	&	1	&	6	&	10	&	48	&	6	\\
    13	&	1	&	19	&	12	&	43	&	8	\\
    14	&	11	&	44	&	11	&	14	&	1	\\
    15	&	8	&	16	&	11	&	25	&	13	\\
    16	&	2	&	41	&	10	&	32	&	15	\\
    17	&	5	&	15	&	14	&	47	&	8	\\
    18	&	8	&	12	&	9	&	16	&	0	\\
    \bottomrule
\end{tabular}
\end{table}

\begin{table}[hbt!]
  \caption{Not using: Number of verbalization segments in each category in ITA}
  \label{tab:numSegITA}
  \begin{tabular}{p{0.3cm}|p{1.35cm}|p{1.4cm}|p{0.8cm}|p{1.2cm}|p{1.0cm}}
    \toprule
    ID & Explanation & Observation & Others & Procedure & Reading\\
    \midrule
    1	&	3	&	12	&	11	&	21	&	6	\\
    2	&	3	&	35	&	25	&	10	&	4	\\
    3	&	18	&	86	&	16	&	29	&	23	\\
    4	&	0	&	23	&	15	&	13	&	6	\\
    5	&	15	&	53	&	27	&	46	&	11	\\
    6	&	7	&	36	&	14	&	32	&	5	\\
    7	&	8	&	47	&	22	&	20	&	32	\\
    8	&	3	&	37	&	22	&	16	&	29	\\
    9	&	1	&	46	&	20	&	36	&	24	\\
    10	&	8	&	47	&	14	&	67	&	8	\\
    11	&	8	&	36	&	16	&	24	&	6	\\
    12	&	7	&	28	&	13	&	16	&	3	\\
    13	&	9	&	44	&	14	&	19	&	9	\\
    14	&	16	&	77	&	16	&	31	&	12	\\
    15	&	20	&	36	&	13	&	34	&	8	\\
    16	&	5	&	28	&	8	&	16	&	12	\\
    17	&	7	&	25	&	16	&	23	&	11	\\
    18	&	23	&	30	&	29	&	83	&	25	\\
    \bottomrule
\end{tabular}
\end{table}

%%Language: Percentage of verbalization units

\begin{table}[hbt!]
  \caption{Not using: Percentage of verbalization units in each category for each participant}
  \label{tab:perSegIndi}
  \begin{tabular}{p{0.3cm}|p{1.35cm}|p{1.4cm}|p{0.8cm}|p{1.2cm}|p{1.0cm}}
    \toprule
    ID & Explanation & Observation & Others & Procedure & Reading\\
    \midrule
1	&	6.9	\%	&	26.9	\% &	20.7	\% &	26.2	\% &	19.3\%	\\
2	&	3.9	\%	&	33.7	\% &	31.8	\% &	26.3	\% &	4.3\%	\\
3	&	5.7	\%	&	40.8	\% &	12.1	\% &	28.7	\% &	12.6\%	\\
4	&	0.5	\%	&	33.0	\% &	22.8	\% &	36.5	\% &	7.1\%	\\
5	&	7.9	\%	&	34.6	\% &	23.6	\% &	20.9	\% &	13.1\%	\\
6	&	5.6	\%	&	26.3	\% &	19.2	\% &	44.4	\% &	4.5\%	\\
7	&	5.1	\%	&	25.1	\% &	18.5	\% &	26.9	\% &	24.4\%	\\
8	&	5.3	\%	&	30.6	\% &	22.5	\% &	23.9	\% &	17.7\%	\\
9	&	2.8	\%	&	46.2	\% &	14.1	\% &	23.7	\% &	13.2\%	\\
10	&	5.8	\%	&	35.8	\% &	14.7	\% &	37.5	\% &	6.1\%	\\
11	&	5.9	\%	&	36.6	\% &	15.7	\% &	35.9	\% &	5.9\%	\\
12	&	5.4	\%	&	24.1	\% &	16.7	\% &	43.3	\% &	10.3\%	\\
13	&	4.6	\%	&	38.2	\% &	17.6	\% &	29.4	\% &	10.1\%	\\
14	&	10.2	\%	&	51.2	\% &	13.9	\% &	18.5	\% &	6.2\%	\\
15	&	11.9	\%	&	25.7	\% &	12.6	\% &	38.3	\% &	11.5\%	\\
16	&	6.5	\%	&	31.9	\% &	12.9	\% &	34.8	\% &	14.0\%	\\
17	&	7.3	\%	&	26.2	\% &	19.4	\% &	36.9	\% &	10.2\%	\\
18	&	11.0	\%	&	22.8	\% &	14.3	\% &	39.3	\% &	12.6\%	\\
    \bottomrule
\end{tabular}
\end{table}

\begin{table}[hbt!]
  \caption{Not using: Percentage of verbalization segments in each category in CTA}
  \label{tab:perSegCTA}
  \begin{tabular}{p{0.7cm}|p{1.35cm}|p{1.4cm}|p{0.8cm}|p{1.2cm}|p{1.0cm}}
    \toprule
    ID & Explanation & Observation & Others & Procedure & Reading\\
    \midrule
1	&	7.3\%	&	32.7\%	&	16.4\%	&	16.4\%	&	27.3\%	\\
2	&	4.3\%	&	22.6\%	&	27.0\%	&	41.7\%	&	4.3\%	\\
3	&	1.2\%	&	39.3\%	&	17.9\%	&	34.5\%	&	7.1\%	\\
4	&	0.0\%	&	43.7\%	&	16.9\%	&	35.2\%	&	4.2\%	\\
5	&	8.5\%	&	37.2\%	&	24.5\%	&	13.8\%	&	16.0\%	\\
6	&	0.0\%	&	7.5\%	&	13.2\%	&	75.5\%	&	3.8\%	\\
7	&	0.0\%	&	12.0\%	&	18.1\%	&	51.8\%	&	18.1\%	\\
8	&	5.7\%	&	41.5\%	&	18.9\%	&	20.8\%	&	13.2\%	\\
9	&	3.2\%	&	43.2\%	&	15.2\%	&	24.8\%	&	13.6\%	\\
Native speakers	&	3.4\%	&	31.8\%	&	19.2\%	&	34.0\%	&	11.6\%	\\
10	&	3.9\%	&	35.0\%	&	19.4\%	&	33.0\%	&	8.7\%	\\
11	&	5.6\%	&	19.1\%	&	15.7\%	&	58.4\%	&	1.1\%	\\
12	&	4.6\%	&	23.1\%	&	16.9\%	&	36.9\%	&	18.5\%	\\
13	&	3.1\%	&	42.2\%	&	21.9\%	&	21.9\%	&	10.9\%	\\
14	&	6.6\%	&	49.5\%	&	19.8\%	&	16.5\%	&	7.7\%	\\
15	&	4.7\%	&	20.0\%	&	11.8\%	&	51.8\%	&	11.8\%	\\
16	&	10.0\%	&	18.2\%	&	16.4\%	&	44.5\%	&	10.9\%	\\
17	&	8.6\%	&	40.0\%	&	28.6\%	&	17.1\%	&	5.7\%	\\
18	&	7.0\%	&	31.8\%	&	10.9\%	&	34.1\%	&	16.3\%	\\
Non-native speakers	&	5.9\%	&	31.0\%	&	17.1\%	&	35.4\%	&	10.5\%	\\
    \bottomrule
\end{tabular}
\end{table}

\begin{table}[hbt!]
  \caption{Not using: Percentage of verbalization segments in each category in SC}
  \label{tab:perSegSC}
  \begin{tabular}{p{0.7cm}|p{1.35cm}|p{1.4cm}|p{0.8cm}|p{1.2cm}|p{1.0cm}}
    \toprule
    ID & Explanation & Observation & Others & Procedure & Reading\\
    \midrule
1	&	8.1\%	&	24.3\%	&	27\%	&	21.6\%	&	18.9\%	\\
2	&	3.2\%	&	39.7\%	&	39.7\%	&	14.3\%	&	3.2\%	\\
3	&	1.1\%	&	25\%	&	12\%	&	45.7\%	&	16.3\%	\\
4	&	1.4\%	&	15.9\%	&	26.1\%	&	49.3\%	&	7.2\%	\\
5	&	5.1\%	&	32.4\%	&	29.4\%	&	15.4\%	&	17.6\%	\\
6	&	7.8\%	&	23.5\%	&	33.3\%	&	31.4\%	&	3.9\%	\\
7	&	9.5\%	&	19\%	&	22.2\%	&	17.5\%	&	31.7\%	\\
8	&	10.2\%	&	10.2\%	&	30.6\%	&	46.9\%	&	2\%	\\
9	&	4.9\%	&	62.1\%	&	10.7\%	&	16.5\%	&	5.8\%	\\
Native speakers	&	5.1\%	&	30.9\%	&	24.3\%	&	27.3\%	&	12.4\%	\\
10	&	10.9\%	&	47.8\%	&	19.6\%	&	19.6\%	&	2.2\%	\\
11	&	3.9\%	&	46.5\%	&	14.2\%	&	26.8\%	&	8.7\%	\\
12	&	1.4\%	&	8.5\%	&	14.1\%	&	67.6\%	&	8.5\%	\\
13	&	1.2\%	&	22.9\%	&	14.5\%	&	51.8\%	&	9.6\%	\\
14	&	13.6\%	&	54.3\%	&	13.6\%	&	17.3\%	&	1.2\%	\\
15	&	11\%	&	21.9\%	&	15.1\%	&	34.2\%	&	17.8\%	\\
16	&	2\%	&	41\%	&	10\%	&	32\%	&	15\%	\\
17	&	5.6\%	&	16.9\%	&	15.7\%	&	52.8\%	&	9\%	\\
18	&	17.8\%	&	26.7\%	&	20\%	&	35.6\%	&	0\%	\\
Non-native speakers	&	6.4\%	&	32.7\%	&	14.5\%	&	37.5\%	&	8.8\%	\\
    \bottomrule
\end{tabular}
\end{table}

\begin{table}[hbt!]
  \caption{Not using: Individual Percentage of verbalization segments in each category in ITA}
  \label{tab:indiperSegITA}
  \begin{tabular}{p{0.7cm}|p{1.35cm}|p{1.4cm}|p{0.8cm}|p{1.2cm}|p{1.0cm}}
    \toprule
    ID & Explanation & Observation & Others & Procedure & Reading\\
    \midrule
1	&	5.7\%	&	22.6\%	&	20.8\%	&	39.6\%	&	11.3\%	\\
2	&	3.9\%	&	45.5\%	&	32.5\%	&	13\%	&	5.2\%	\\
3	&	10.5\%	&	50\%	&	9.3\%	&	16.9\%	&	13.4\%	\\
4	&	0\%	&	40.4\%	&	26.3\%	&	22.8\%	&	10.5\%	\\
5	&	9.9\%	&	34.9\%	&	17.8\%	&	30.3\%	&	7.2\%	\\
6	&	7.4\%	&	38.3\%	&	14.9\%	&	34\%	&	5.3\%	\\
7	&	6.2\%	&	36.4\%	&	17.1\%	&	15.5\%	&	24.8\%	\\
8	&	2.8\%	&	34.6\%	&	20.6\%	&	15\%	&	27.1\%	\\
9	&	0.8\%	&	36.2\%	&	15.7\%	&	28.3\%	&	18.9\%	\\
Native speakers	&	6.0\%	&	38.7\%	&	17.8\%	&	23.0\%	&	14.5\%	\\
10	&	5.6\%	&	32.6\%	&	9.7\%	&	46.5\%	&	5.6\%	\\
11	&	8.9\%	&	40\%	&	17.8\%	&	26.7\%	&	6.7\%	\\
12	&	10.4\%	&	41.8\%	&	19.4\%	&	23.9\%	&	4.5\%	\\
13	&	9.5\%	&	46.3\%	&	14.7\%	&	20\%	&	9.5\%	\\
14	&	10.5\%	&	50.7\%	&	10.5\%	&	20.4\%	&	7.9\%	\\
15	&	18\%	&	32.4\%	&	11.7\%	&	30.6\%	&	7.2\%	\\
16	&	7.2\%	&	40.6\%	&	11.6\%	&	23.2\%	&	17.4\%	\\
17	&	8.5\%	&	30.5\%	&	19.5\%	&	28\%	&	13.4\%	\\
18	&	12.1\%	&	15.8\%	&	15.3\%	&	43.7\%	&	13.2\%	\\
Non-native speakers	&	10.3\%	&	35.1\%	&	13.9\%	&	31.3\%	&	9.4\%	\\
    \bottomrule
\end{tabular}
\end{table}

%Language_Part 3: Problems
\begin{table}[hbt!]
  \caption{Not using: Individual number of occurrences of usability problems identified from analyzing verbalization units}
  \label{tab:indiup}
  \begin{tabular}{cc}
    \toprule
ID	&	No. of problems	\\
    \midrule
1	&	3	\\
2	&	4	\\
3	&	10	\\
4	&	4	\\
5	&	5	\\
6	&	1	\\
7	&	3	\\
8	&	1	\\
9	&	5	\\
Native speakers	&	36	\\
10	&	5	\\
11	&	12	\\
12	&	3	\\
13	&	3	\\
14	&	4	\\
15	&	4	\\
16	&	5	\\
17	&	2	\\
18	&	4	\\
Non-native speakers	&	42	\\
Total	&	78	\\
    \bottomrule
\end{tabular}
\end{table}

%hi yea haha, i'll do it later haha
%some tablesa are not being used tho
%okie~ thank you! i'll come back later Sure. 
%nice meeting u here haha
% are you working in the doc now? OK. I try to format all the tables to two-column formats. You can come back and work on it. 
%yeah, I realize that. Also many tables need to be condensed. But I just want to go through all in one pass without having to worry about which is used and which is not
% I think there is a chat function in overleaf. On the top right corner, we can chat there in the future. But we can always use Slack. See you later.
%see ya~~:)
